# Supplementary material for: Quantum Hall Effect, Screening and Layer-Polarized Insulating States in Twisted Bilayer Graphene
Source: arXiv:1110.4628 ancillary file (2011-10-20)
Supplement: Supplementary file 1 [file Sanchez-QHETwistedBilayer_Supp.pdf]

# Supplementary Information: Quantum Hall Effect, Screening and Layer-Polarized Insulating States in Twisted Bilayer Graphene

Javier D Sanchez-Yamagishi,[1,*] Thiti Taychatanapat,[2,*] Kenji Watanabe,[3]
Takashi Taniguchi,[3] Amir Yacoby,[2] and Pablo Jarillo-Herrero[1]

[1]*Department of Physics, Massachusetts Institute of Technology, Cambridge, MA 02139 USA*

[2]*Department of Physics, Harvard University, Cambridge, MA 02138 USA*

[3]*National Institute for Materials Science, Namiki 1-1, Tsukuba, Ibaraki 305-0044, Japan*

(Dated: October 20, 2011)

## CONTENTS

Sample Fabrication 2

Contact Geometry 3

Displacement Field, Density and Screening 3

Background Subtraction 5

Consistency Between Zero and High Magnetic Field Measurements 6

References 6

## SAMPLE FABRICATION

Our twisted bilayer graphene samples were fabricated on a hexagonal Boron Nitride (h-BN) substrate, using the same PMMA-transfer technique described by Taychatanapat *et al.* [1]. Flakes of h-BN were used as substrates for the twisted bilayer graphene to ensure high sample quality and low impurity doping [2, 3]. First, h-BN was mechanically exfoliated onto Si substrates with 285 nm of thermally grown oxide, and then flat h-BN flakes were identified using optical and atomic force microscopy. Two graphene sheets were then sequentially transferred to the same h-BN flake such that they overlap to form a bilayer region. Because we cannot determine or control the crystallographic orientation of the graphene sheets, the transfer process results in a random twist angle between the lattices of the two graphene layers. Atomic force microscopy measurements indicate a step height between the layers that varies from 3.4 to 4.1 Å across three different samples, which is very close to the inter-layer distance of 3.4 Å observed in graphite [4].

Next, the graphene layers are lithographically patterned and then etched in an Oxygen reactive ion etcher to isolate the overlapping region where the twisted bilayer graphene is formed. The isolated twisted bilayer graphene is then contacted using thermally evaporated Cr/Au. Finally, a topgate is made by transferring a thin h-BN flake on top of the contacted twisted bilayer graphene, followed by the fabrication of additional Cr/Au contacts for the topgate electrodes.

After each step where the graphene encounters PMMA or solvents the entire device is heat annealed for 3 hours at 350°C under Ar and H flow.

## CONTACT GEOMETRY

In this work, twisted bilayer graphene was made by stacking two monolayer graphene sheets which overlap to form a bilayer region. For these samples, the monolayer graphene sheets extend beyond the overlap region, allowing for metal electrodes to be deposited which only contact one of the layers. We find that current flows freely between the layers: measuring the resistance of the overlap region with probes on separate layers shows no measurable increase compared to probes on the same layer. In addition, inter-layer current vs voltage measurements are found to be linear down to 0.1 mV. The net result is that we see no layer-specific effects due to our contact geometry and we treat the probes as contacting the bilayer as a single unit.

## DISPLACEMENT FIELD, DENSITY AND SCREENING

This work focuses on the magnetoresistance of twisted bilayer graphene as a function of the total carrier density on the bilayer and the displacement field applied normal to the layers. As stated in the main text, the total density $n_{\mathrm{tot}}$ and displacement field $D$ are given as follows:

$$en_{\mathrm{tot}} = (C_{\mathrm{T}}V_{\mathrm{TG}} + C_{\mathrm{B}}V_{\mathrm{BG}}),\ D = (C_{\mathrm{T}}V_{\mathrm{TG}} - C_{\mathrm{B}}V_{\mathrm{BG}})/2, \tag{S1}$$

where $e$ is the elementary charge, $C_{\mathrm{T(B)}}$ is the capacitance per unit area to ground of the top (bottom) gate, and $V_{\mathrm{TG(BG)}}$ is the potential difference between the top (bottom) gate and the graphene layer closest to it. This potential difference will be primarily determined by the voltage $V_{\mathrm{T(B)}}$ applied to the top (bottom) gate, with a small correction due to the graphene chemical potential as: $V_{\mathrm{TG}} = V_{\mathrm{T}} - \mu_{\mathrm{U}}$ and $V_{\mathrm{BG}} = V_{\mathrm{B}} - \mu_{\mathrm{L}}$, where $\mu_{\mathrm{U(L)}}$ is the chemical potential of the upper (lower) graphene layer.

The value of $\mu_{\mathrm{U(L)}}$ in response to the applied gate voltages will be determined by the inter-layer screening and charging behavior as the bilayer responds to the applied field $D$, while keeping $n_{\mathrm{tot}}$ as given in equation S1. As discussed in the main text, $D$ will be screened

by the layer density imbalance as well as the inter-layer dielectric environment. The resulting chemical potential difference between the two layers is given by the following equation:

$$C_{\rm GG}\frac{(\mu_{\rm U}-\mu_{\rm L})}{e} = D - e\frac{(n_{\rm U}-n_{\rm L})}{2}, \tag{S2}$$

where $n_{\rm U(L)}$ is the carrier density on the upper (lower) layer and $C_{\rm GG}$ is the inter-layer capacitance.

The graphene chemical potential at zero magnetic field is given by $\mu = \hbar v_F\sqrt{\pi n}$ [5], where $n$ is the density of the monolayer graphene sheet, $\hbar$ is the reduced Planck constant and $v_F$ is the graphene Fermi velocity. Although the density dependence of $\mu$ will change in a magnetic field due to Landau level (LL) formation, this formula will still hold when the chemical potential lies at the graphene LL energy, and in most cases offers a better approximation than completely neglecting the chemical potential term.

The above equations can be solved numerically to produce a relation between the applied gate voltages and the chemical potential of the graphene sheets, as well as the actual value of

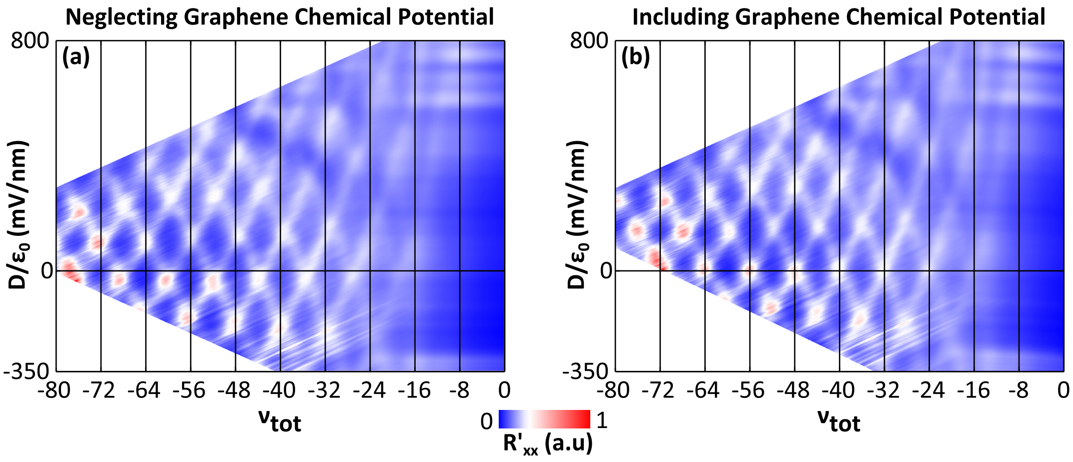


FIG. S1. (a) Background subtracted longitudinal resistance $R'_{\rm xx}$ at $B$=4T, as a function of the displacement field $D$ and filling factor $\nu_{\rm tot}$, neglecting the graphene chemical potential. The layer degenerate crossings do no occur at $D = 0$ and the filling factors do not match the correct crossings. (b) Same $R'_{\rm xx}$, but with $D$ and $\nu_{\rm tot}$ calculated to include the graphene chemical potential and the screening properties of the twisted bilayer. Layer degenerate crossings now occur at $D = 0$ and at integer multiples of filling factor 8. The plot in (b) is the same data that appears in Figure 2f of the main text.

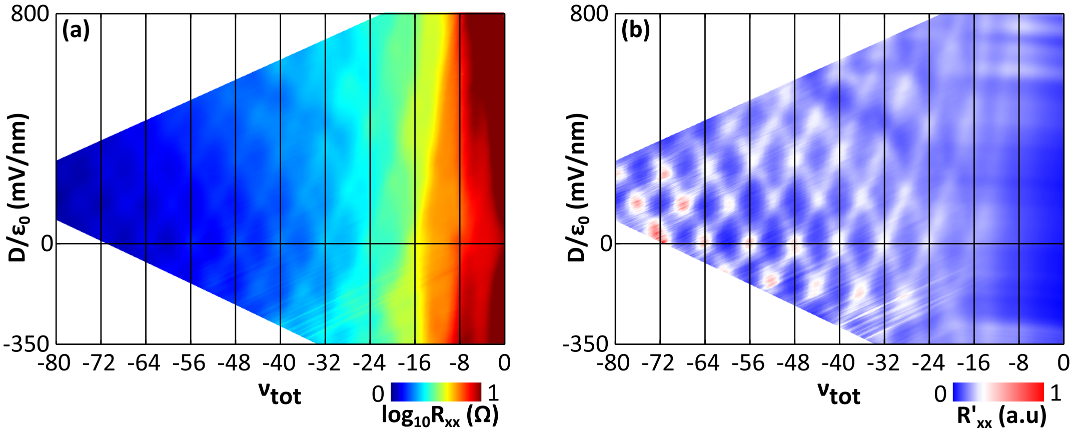


FIG. S2. (a) Longitudinal resistance $R_{\mathrm{xx}}$ as a function of displacement field $D$ and total filling factor $\nu_{\mathrm{tot}}$ with log color scale. (b) Same data from (a), but with smooth background subtracted. Crossings visible in (b) occur in the same location as in (a).

$n_{\mathrm{tot}}$ and $D$ which are used throughout the paper. The importance of the chemical potential terms can be seen in Figure S1, where the background subtracted longitudinal resistance is plotted as a function of $D$ and $\nu_{\mathrm{tot}} = n_{\mathrm{tot}}h/eB$, without the chemical potential correction (Fig. S1a), and with the chemical potential correction (Fig. S1b). For the uncorrected values, the layer degenerate crossings do not match $D = 0$, and do not occur at the right filling factors. Taking into account the chemical potential terms and the inter-layer screening results in more accurate values for $n_{\mathrm{tot}}$ and $D$ (Fig. S1b), with the layer degenerate crossings occurring at $D = 0$ and at integer multiples of filling factor 8.

## BACKGROUND SUBTRACTION

In Figure 2f we present a longitudinal resistance measurement $R_{\mathrm{xx}}$ with the background subtracted. This is done to increase the contrast of local $R_{\mathrm{xx}}$ peaks which correspond to the Fermi energy lying within a Landau level. This background subtraction was performed by removing a linear fit from $1/R_{\mathrm{xx}}$ and then scaling uniformly for high color contrast. As can be seen in Figure S2b, the peaks in the background subtracted $R'_{\mathrm{xx}}$ occur in the same location as the original $R_{\mathrm{xx}}$ measurement in Figure S2a.

## CONSISTENCY BETWEEN ZERO AND HIGH MAGNETIC FIELD MEASUREMENTS

We now show that our zero magnetic field measurements (Figure 1d) are consistent with our high-field data and inter-layer screening model. At the charge neutrality point (CNP), where $n_{\text{tot}} = 0$, the resistance is observed to decrease with increasing $D$, and at the highest displacement fields ($D/\epsilon_0$=900 mV/nm) a small splitting of the resistance peak begins to develop. From our high field measurements we know that the effect of $D$ is to induce density imbalances between the two layers. For the case where $n_{\text{tot}} = 0$, this density imbalance must result in equal but opposite sign charge densities on the two layers. Each individual layer then is doped away from its CNP, lowering its resistance, and in turn lowering the parallel resistance of the two layers. At high enough D, the density difference between the layers should be large enough to separately resolve the CNP of each layer. For the case of the device in Figure 1d, a splitting of the resistance peak by $\Delta n_{\text{tot}} = 6 \times 10^{11}$ cm$^{-2}$ is observed at $D/\epsilon_0$=900 mV/nm. This corresponds to a chemical potential difference of $\Delta\mu = 128$ meV between the two layers. Applying equation S2 to these values for $D$, $\Delta n_{\text{tot}}$ and $\Delta\mu$ results in a value for the interlayer capacitance of $C_{\text{GG}} \sim 6$ $\mu$F/cm$^{-2}$. This value is very similar to that extracted from our high magnetic field analysis of the same sample ($C_{\text{GG}} = 6.8$ $\mu$F/cm$^2$), and shows that the screening analysis is consistent for zero and high magnetic fields.

---

* These authors contributed equally to this work

[1] T. Taychatanapat, K. Watanabe, T. Taniguchi, and P. Jarillo-Herrero, Nat. Phys. **7**, 621 (2011).

[2] C. R. Dean *et al.*, Nat. Nanotechnol. **5**, 722 (2010).

[3] J. Xue *et al.*, Nat. Mater. **10**, 282 (2011).

[4] M. S. Dresselhaus and G. Dresselhaus, Adv. Phys. **51**, 1 (2002).

[5] A. H. Castro Neto *et al.*, Rev. Mod. Phys. **81**, 109 (2009).
